# Supplementary material for: New Giant Planet beyond the Snow Line for an Extended MOA Exoplanet Microlens Sample
Source: arXiv:2107.03400 source file (2021-07-07)
Supplement: Supplementary file 1 [file aastex63_additional_journal_abbreviations.tex]

\newcommand\cse{\ref@jnl{CSE}}%     %  Computing In Science Engineering %%CR Added
